# Supplementary material for: KohakuRAG: A simple RAG framework with hierarchical document indexing
Source: arXiv:2603.07612 source file (2026-03-08)
Supplement: Supplementary file 1 [file author_contribution.tex]

\section{Author Contributions}
\label{app:contributions}

Table~\ref{tab:contributions} summarizes the contributions of each author across four categories: algorithm design, system development, experimentation, and paper writing. Each column distributes 10 contribution points among authors.

\begin{table}[H]
\centering
\caption{Author contributions across different aspects of the project. Each column sums to 10 points.}
\label{tab:contributions}
\begin{tabular}{lcccc}
\toprule
\textbf{Author} & \textbf{Algorithm} & \textbf{Development} & \textbf{Experiments} & \textbf{Writing} \\
\midrule
Shih-Ying Yeh   & **** & ****** & *** & **** \\
Yueh-Feng Ku    & **   & **   & *** & **   \\
Ko-Wei Huang    & **   & *   & **  & **   \\
Buu-Khang Tu    & **   & *   & **  & **   \\
\bottomrule
\end{tabular}
\end{table}
